# Supplementary material for: Quantum Valley and Sub-valley Hall Effect in the Large Angle Twisted Bilayer Graphene
Source: arXiv:2306.02655 source file (2023-09-12)
Supplement: Supplementary file 1 [file supplimental.tex]

\def\n{\noindent}
\def\RMP{{Rev. Mod. Phys.\ }\/}
\def\PRL{{ Phys. Rev. Lett.\ }\/}
\def\PRB{{ Phys. Rev. B\ }\/}
\def\PRX{{ Phys. Rev. X\ }\/}
\def\etal{{\it et al.~}\/}
\def\eq{\ =\ }
\def\dpr{^{\prime\prime}}
\newcommand{\angstrom}{\AA}
\makeatletter
\newcommand{\rmnum}[1]{\romannumeral #1}
\newcommand{\Rmnum}[1]{\expandafter\@slowromancap\romannumeral #1@}
\newcommand{\uvec}[1]{\boldsymbol{\hat{\textbf{#1}}}}
\makeatother

\makeatletter
\newcommand*\env@matrix[1][*\c@MaxMatrixCols c]{%
  \hskip -\arraycolsep
  \let\@ifnextchar\new@ifnextchar
  \array{#1}}
\makeatother

\documentclass[aps,prb,showpacs,superscriptaddress,a4paper,twocolumn]{revtex4-2}
%\documentclass[a4paper,12pt, english]{article}
\usepackage{amsmath}
\usepackage{float}
%\usepackage{MnSymbol}
\usepackage{color}
%\input{rgb}

\usepackage{mathtools}
\usepackage{textcmds}
\usepackage{braket}

%\usepackage{physics}

\usepackage[normalem]{ulem}
\usepackage{soul}
\usepackage{amssymb}

\usepackage{amsfonts}
\usepackage{amssymb}
%\usepackage[showframe]{geometry}% http://ctan.org/pkg/geometry
%\usepackage{lipsum}% http://ctan.org/pkg/lipsum
\usepackage{graphicx}
%\usepackage{caption}
\parskip 0.1cm
\voffset 0.5cm



\newcommand{\beginsupplement}{%
        \setcounter{table}{0}
        \renewcommand{\thetable}{S\arabic{table}}%
        \setcounter{figure}{0}
        \renewcommand{\thefigure}{S\arabic{figure}}%
     }


\makeatletter
\renewcommand \thesection{S\@arabic\c@section}
\renewcommand\thetable{S\@arabic\c@table}
\renewcommand \thefigure{S\@arabic\c@figure}
\renewcommand \theequation{S\@arabic\c@equation}
\makeatother

\newcommand{\overbar}[1]{\mkern 1.5mu\overline{\mkern-1.5mu#1\mkern-1.5mu}\mkern 1.5mu}

\newcommand{\red}[1]{{\textcolor{red}{#1}}}
\newcommand{\blue}[1]{{\textcolor{blue}{#1}}}
\newcommand{\magenta}[1]{{\textcolor{magenta}{#1}}}
\newcommand{\ma}{\sigma}
\newcommand{\V}{\vec}
\newcommand{\dt}{\delta}
\newcommand{\ep}{\epsilon}
\newcommand{\f}{\frac}
\newcommand{\ta}{\theta}
\newcommand{\Om}{\Omega}
\newcommand{\pa}{\partial}
\newcommand{\Dt}{\Delta}
\newcommand{\da}{\dagger}
\newcommand{\kb}{\mathbf{k}}
\newcommand{\Mb}{\mathbf{M}}
\newcommand{\Hb}{\mathbf{H}}
\newcommand{\Db}{\mathbf{D}}
\newcommand{\Sb}{\mathbf{S}}
\newcommand{\Bb}{\mathbf{B}}
\newcommand{\db}{\mathbf{d}}
\newcommand{\jb}{\mathbf{j}}
\newcommand{\Fb}{\mathbf{F}}
\newcommand{\vb}{\mathbf{v}}
\newcommand{\Omb}{\mathbf{\Omega}}
\renewcommand{\thefigure}{\arabic{figure}}
\renewcommand{\thetable}{\arabic{table}}
\renewcommand{\thesection}{\arabic{section}}
\renewcommand{\arraystretch}{1.5}
\setlength{\tabcolsep}{3pt}
\newcommand{\sr}[1]{\red{\sout{#1}}}

\begin {document}

\beginsupplement




%%%%%%%%%%%%%%%%%%%%%%%%%%%%%%%%%%%%%%%%%%%%%%%%%
%               TITLE 
%%%%%%%%%%%%%%%%%%%%%%%%%%%%%%%%%%%%%%%%%%%%%%%%%

\title{Supplemental Material for \qq{Quantum Valley and Sub-valley Hall Effect in the Large Angle Twisted Bilayer Graphene} }


\author{Chiranjit Mondal}

\author{Rasoul Ghadimi}

\affiliation{Department of Physics and Astronomy, Seoul National University, Seoul 08826, Korea}
\affiliation{Center for Theoretical Physics (CTP), Seoul National University, Seoul 08826, Korea}

\author{Bohm-Jung Yang}
\email{bjyang@snu.ac.kr}

\affiliation{Department of Physics and Astronomy, Seoul National University, Seoul 08826, Korea}
\affiliation{Center for Theoretical Physics (CTP), Seoul National University, Seoul 08826, Korea}
\affiliation{Center for Correlated Electron Systems, Institute for Basic Science (IBS), Seoul 08826, Korea}

\date{\today}

\maketitle 

%\hfill \\
\twocolumngrid

\tableofcontents

% \newpage


\section*{S1. DFT computational details}
First principle calculations were carried out using projector augmented wave (PAW)\cite{PEBLOCH1994} formalism based on Density Functional Theory (DFT) as implemented in the Vienna ab-initio Simulation Package (VASP).\cite{Hafner1993,Joubert1999} 
The generalized-gradient approximation by Perdew-Burke- Ernzerhof (PBE)\cite{Joubert1999} was employed to describe the exchange and correlation. 
An energy cut-off of 500 eV is used to truncate the plane-wave basis sets. 
The Brillouin zone (BZ) is integrated using 6$\times$6$\times$1 $\Gamma-$centered k-mesh.
DFT-D2 method has been applied for Van der Waals forces correction. 
Tight-binding (TB) Hamiltonians were constructed using maximally localized Wannier functions (MLWFs)\cite{mlwf1,mlwf2,mlwf3} obtained from Wannier90 package\cite{w90}.


\section*{S2. Proposed device geometry}
 We propose a schematic device geometry for the experimental realization of various types of domain wall states under the electric field and (or) stacking geometry reversal between EAB, EBA, and EAA configurations as shown in Fig.~\ref{fig-s1}. 
 The gate in green color represents the $+E$ electric file whereas the orange color represents the $-E$ electric field. 
A domain wall can be created by $E$-field reversal (i.e. by controlling the gate biased) in EAB which consists of two counter-propagating domain wall modes per valley i.e. a total of four domain wall modes as shown by the arrows. 
A domain wall can also be created by creating a junction between EAB/EBA and EAA with the same sign of electric field on both sides of the junction. 
 In this case, domain walls contain one counter-propagating mode per valley (a total of two domain wall modes) as shown by the arrows. 

%%%%%%%%%%%%%%%%%%%%%%%%%%%%%%%%%%%%%%%%%%%%%%%%%%%%%%%
%%======= device  ===========% 
\begin{figure}[t!]
	\centering
	\includegraphics[width=0.5\textwidth]{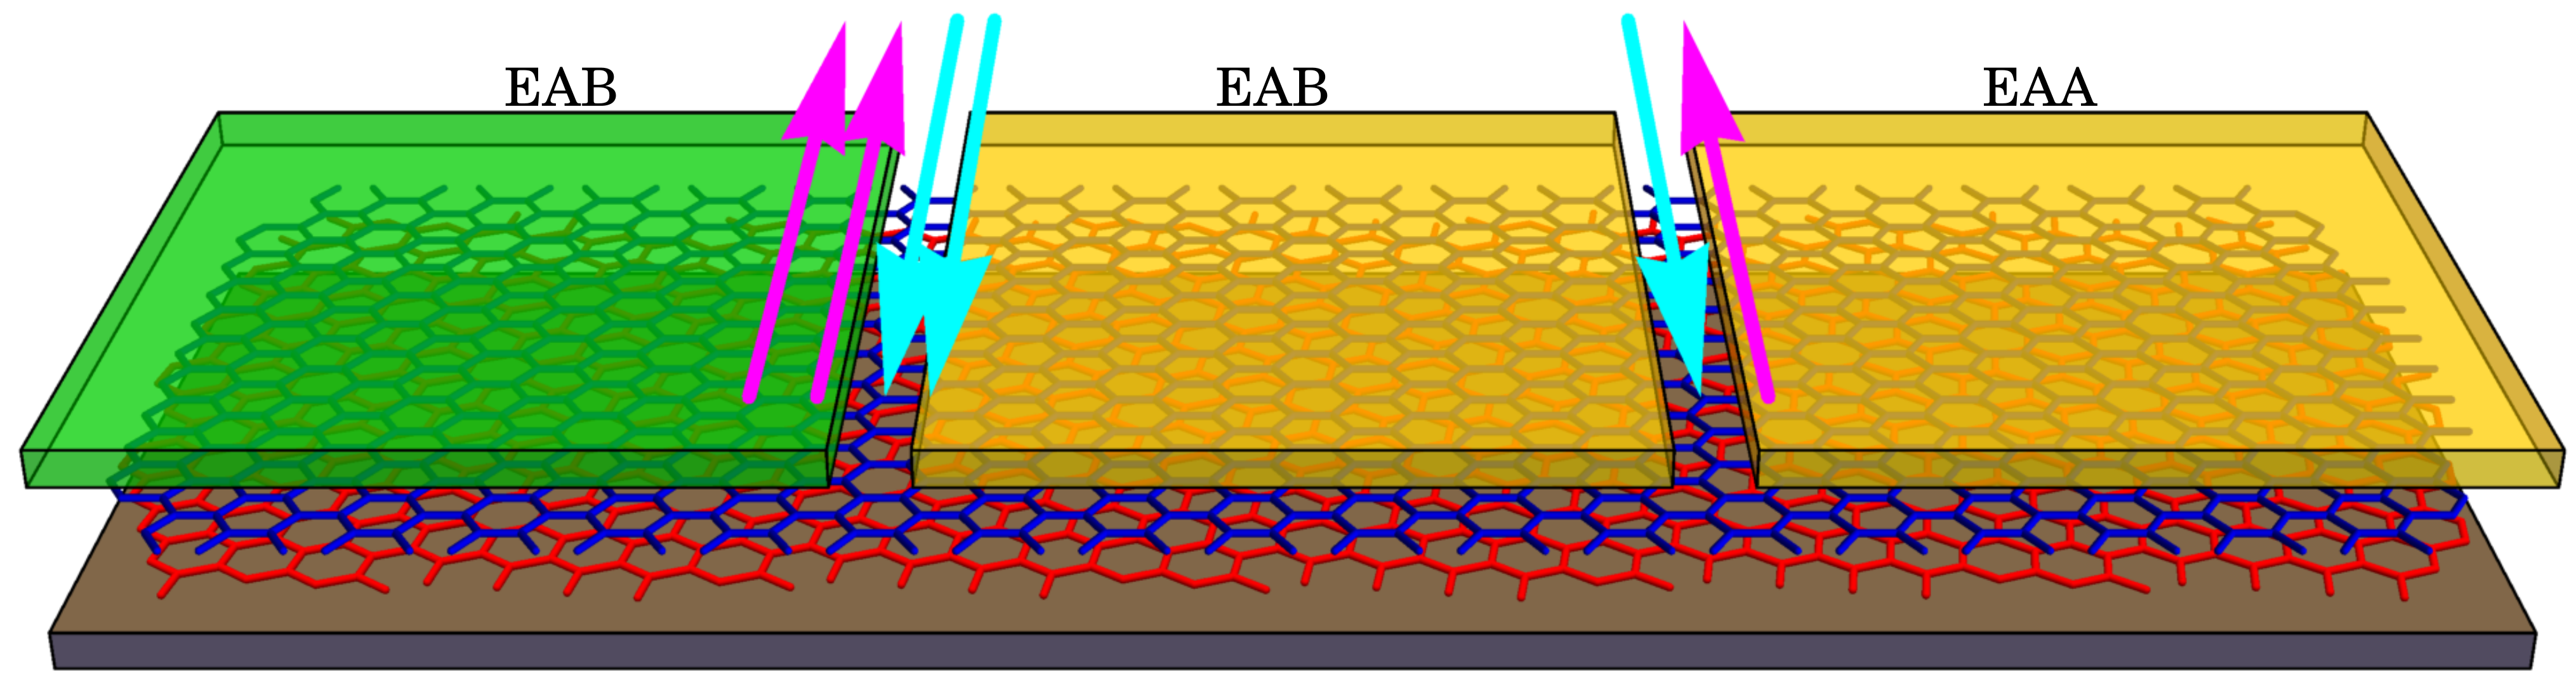}
	\caption{  A schematic device geometry to realize the proposed domain wall states. 
	The gates to apply the positive (negative) $+E$ ($-E$) field are indicated by green (orange) colors. 
	A domain wall is created by alternate gate biased ($+E$ and $-E$) in EAB, which consists of two chiral modes per valley (as shown by the arrows).
	 Another domain wall is created by creating a junction between EAB and EAA under an electric $-E$ which gives one chiral mode per valley.
	  Modes belonging to the opposite valleys are counter-propagating in nature }
	\label{fig-s1}
\end{figure}
%%============================% 
%%%%%%%%%%%%%%%%%%%%%%%%%%%%%%%%%%%%%%%%%%%%%%%%%%%%%%%%%%


\section*{S3. Detail of tight-binding calculation }
We construct a ribbon with 5000 unit cells long along the non-periodic direction. Then we numerically confirm the existence of domain wall and edge modes using a tight-binding Hamiltonian for a ribbon of TBG with $p_z$ orbitals. 
The Hamiltonian is written as, 

\begin{equation}
H=\sum_{<i,j>} t({\bf r}_i - {\bf r}_j) \ket{r_i}\bra{r_j} + h.c
\end{equation}

{\bf r$_i$} represents the position of $i^{th}$ lattice site and $t(\bf r_i - \bf r_j)$ is the  hoping between $i^{th}$ and $j^{th}$ sites which is given by\cite{tbg1,tbg2}
\begin{equation}
 -t({\bf r}) = V_{\pi} \bigl[ 1 - \bigl( \frac{\bf r \cdot e_z }{r}  \bigr)^2 \bigr] + V_{\sigma} \bigl( \frac{\bf r \cdot e_z }{r}  \bigr)^2 .
\end{equation} 
Here, ${\bf r = r_i - r_j}$, $V_{\pi} = V_{\pi}^0 e^{-(\frac{r-a_0}{\delta_0})}$, $V_{\sigma} = V_{\sigma}^0 e^{-(\frac{r-d_0}{\delta_0})}$, 
$a_0 =1.42 \angstrom$  and $a_0 =3.35 \angstrom$  is graphene bond length and bilayer spacing, $V_{\pi}^0$ and $V_{\sigma}^0$ represent the transfer integral between the sites of intralayer and interlayer atoms whose values have been chosen as -2.7 eV and 0.48 eV. $ \delta_0 = 0.318 a_0 $ is the decay length. 


\section*{S4. Shift-dependent effective  Hamiltonian }
The effective low-energy Hamiltonian comprises two parts in TBG, inter-layer and intra-layer part. 
The intra-layer part can be represented by the Dirac Hamiltonian $H_1 (H_2) = -i\nu \sigma \cdot {\bf k}$ ($-i\nu \sigma^\theta_c \cdot {\bf k} $) where $\nu$ is the Fermi velocity, $\sigma = \{\sigma_x, \sigma_y\}$ and $\sigma^\theta = (e^{-i\theta_c \sigma_z} \{\sigma_x, \sigma_y\} e^{i\theta_c \sigma_z})$. 
$H_1$ ($H_2$) is Dirac Hamiltonian corresponding to the unrotated and the rotated layer respectively. 
We write the intra-layer part for both the layers as, $H_{1,2} = -i\nu \sigma \cdot  \nabla = -i\nu (\sigma_x k_x+\sigma_y k_y) $. 
To do this, we make a gauge transformation to the inter-layer Hamiltonian part as,  $H_{inter} \rightarrow H_{inter} ~ e^{-i\sigma_z \theta_c/2}$.


The interlayer coupling part of the Hamiltonian is written as,
\begin{equation}  \label{eq1}
H_{R_i, \tilde{R}_j}^{\alpha,\beta} = \sum_{R_i, \tilde{R}_j} t(R_i + \tau_\alpha - \tilde{R}_j - \tilde{\tau}_\beta ) \ket{R_i, \alpha} \bra{R_j, \beta}
 \end{equation} 
 where $t(R_i + \tau_\alpha - \tilde{R}_j - \tilde{\tau}_\beta )$ represents the inter-layer tunneling amplitude,
  $\alpha, \beta$ represent the sub-lattice index with positions $\tau_i (i=\alpha, \beta)$ for two layers respectively. 
Then we go to the momentum space by doing a Fourier transform as,
\begin{equation} 
\ket{R_i,\alpha} = \sum_{\bf k} e^{-i {\bf k}\cdot {\bf R_i}  } \ket{\phi_{k,\alpha}}
 \end{equation} 
 and,
\begin{equation} 
\ket{\tilde{R}_j, \tilde{\beta} } = \sum_{\bf \tilde{k} } e^{-i {\bf \tilde{k}}\cdot {\bf \tilde{R}_i}  } \ket{\phi_{k,\alpha}}
 \end{equation} 
 The inter-layer part for a general $\theta_c$ becomes,
 \begin{equation}  \label{eq1}
 H_{\bf k,\tilde k}^{\alpha \beta} = \sum_{ \bf G,\tilde G } t_{\bf k+G} e^{i \bf G\cdot (\tau^\alpha + d)} e^{-i \bf \tilde G \cdot\tau^\beta} \delta_{ \bf k+G,\tilde k + \tilde G } ,
 \end{equation} 
 where ${\bf G} = \sum {n_i {\bf b_i} } $ and ${\bf \tilde{G} } = \sum{ \tilde{n_i} {\bf \tilde{b_i} } } $ are the reciprocal lattice vectors for the two layers, respectively, and $t_{\bf k+G}$ is the Fourier coefficient of the tight-binding hopping in the momentum space whose amplitude depends on $|{\bf k+G}|$.
 The coupling Hamiltonian becomes non-zero only when momentum conservation condition ${\bf k+G } = {\bf \tilde{k} + \tilde{G} }$ is satisfied. 

%%%%%%%%%%%%%%%%%%%%%%%%%%%%%%%%%%%%%%%%%%%%%%%%%%%%%%%
%%======= moier theory  ===========% 
\begin{figure}[t!]
	\centering
	\includegraphics[width=0.4\textwidth]{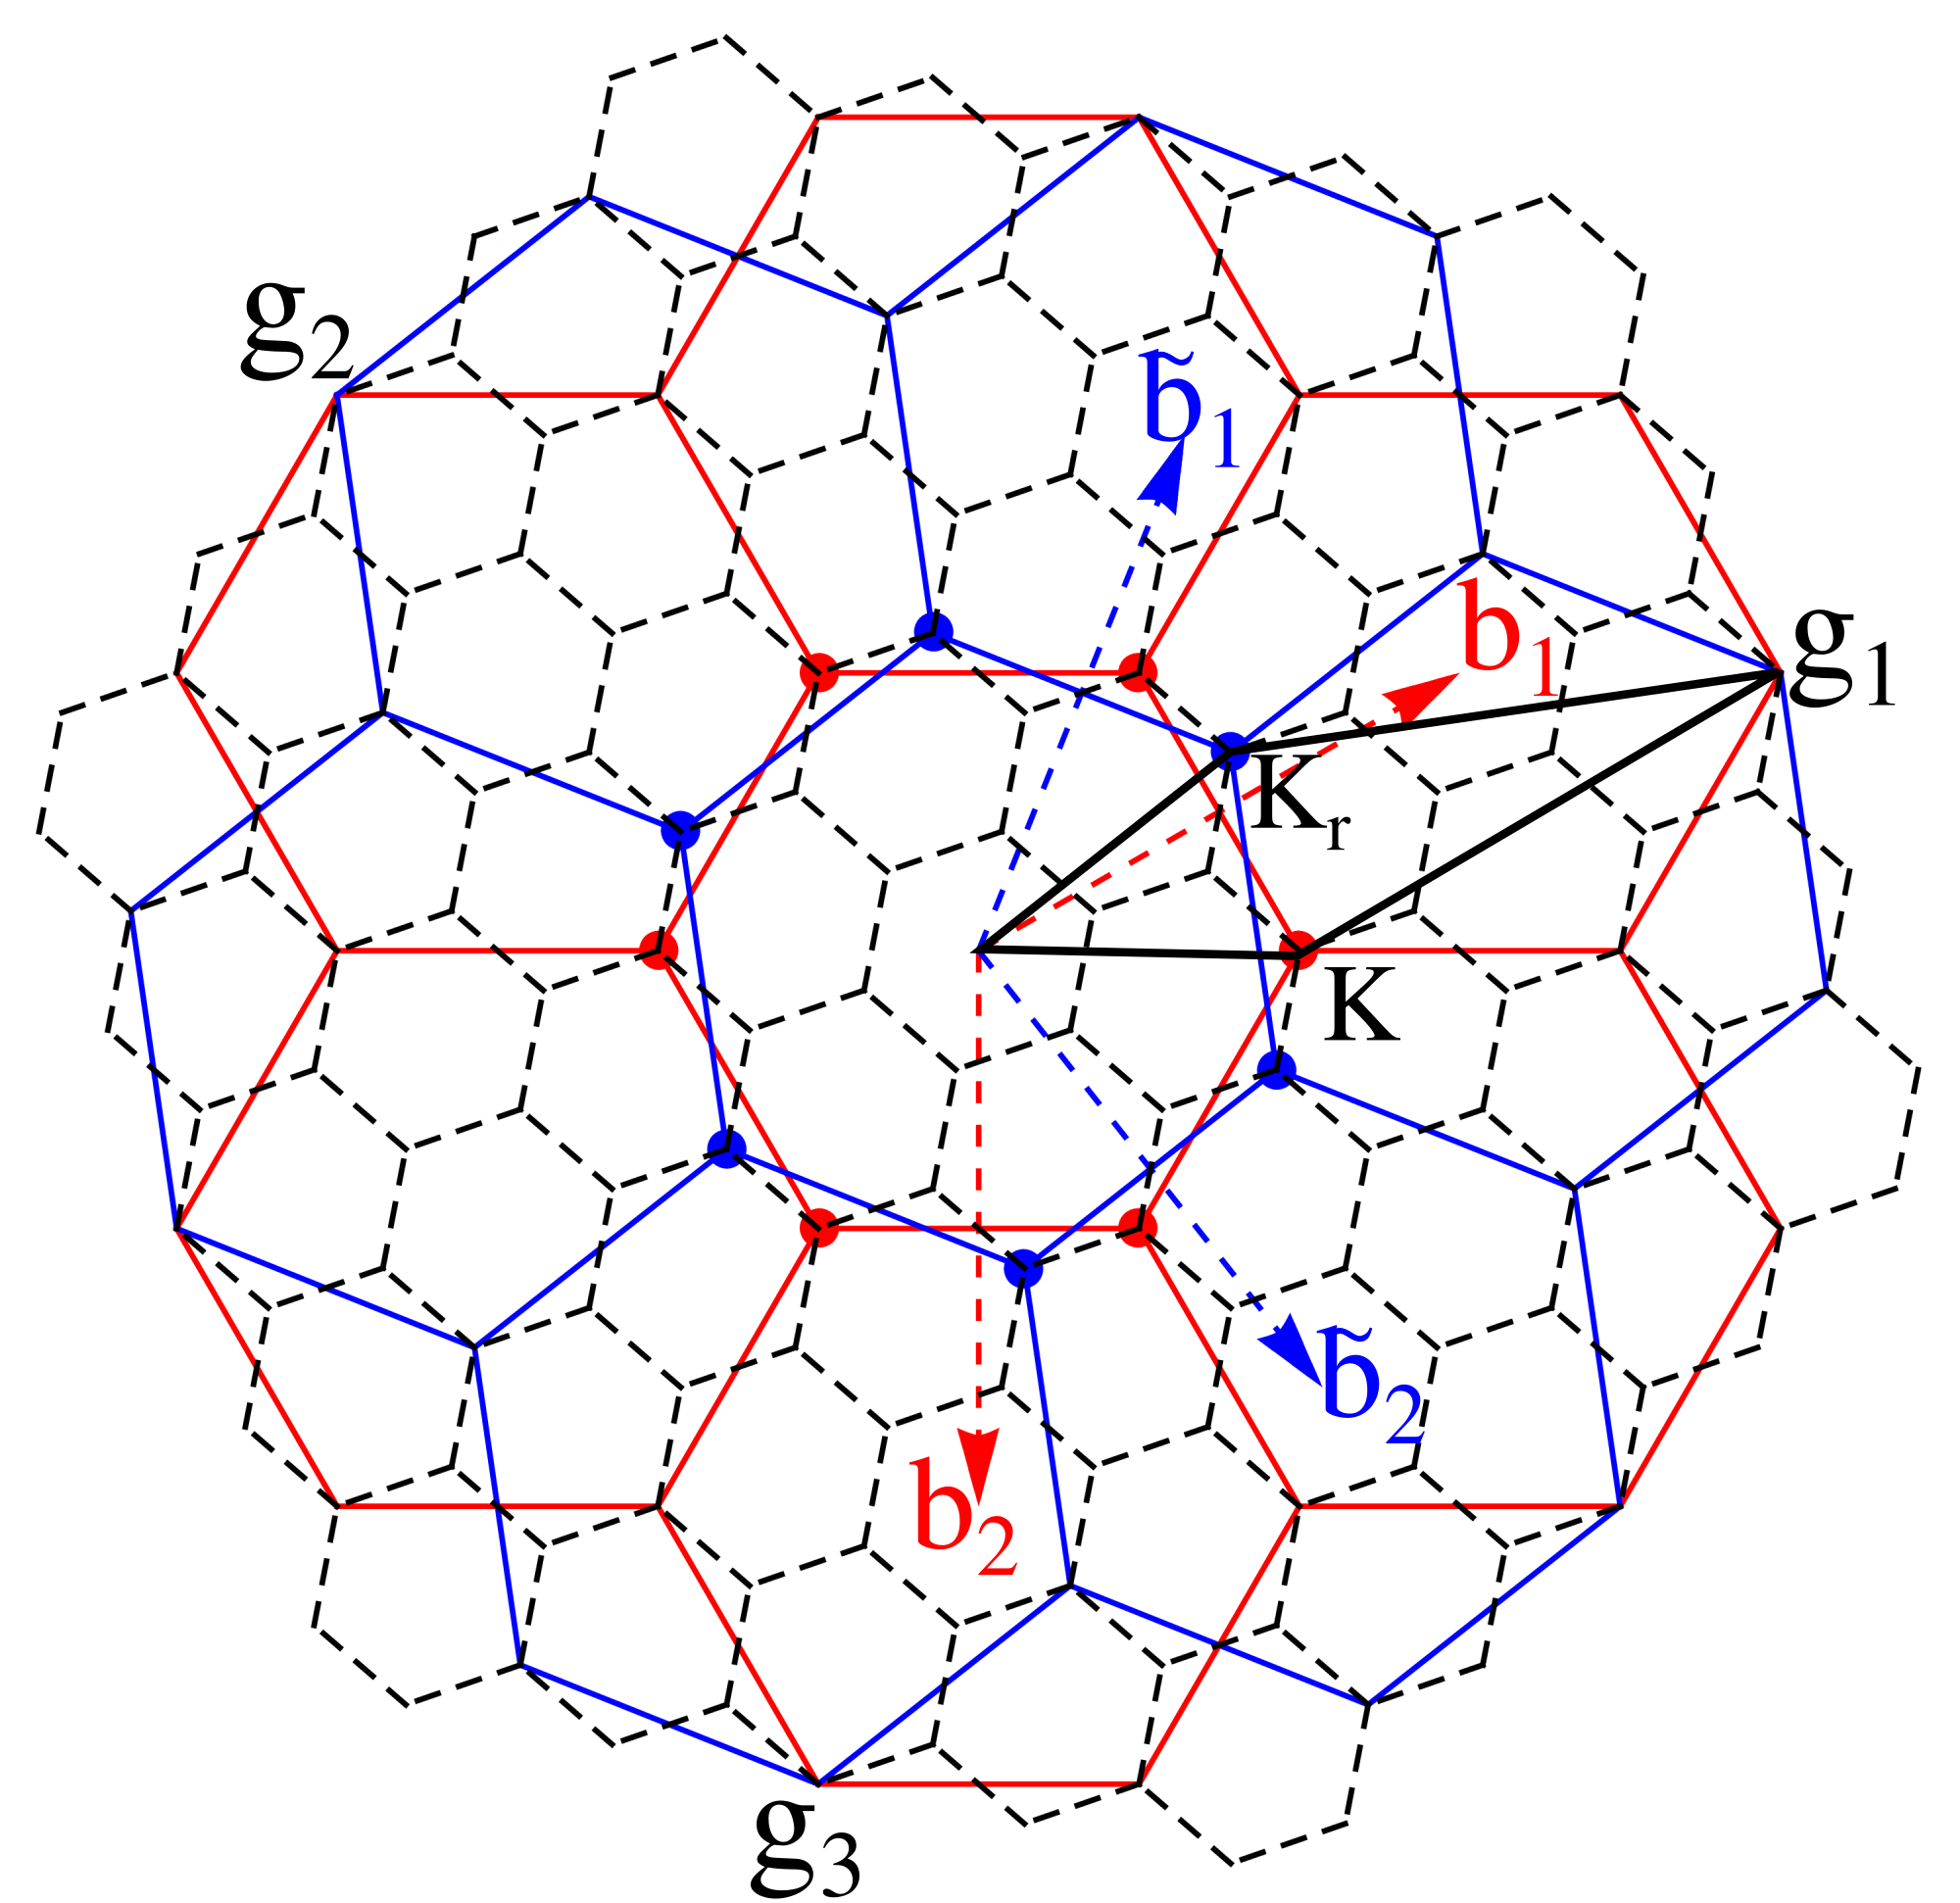}
	\caption{ Brillouin zone (BZ) of a TBG with $\theta_c = 38.21^\circ$. Red and Blue represent the BZ of the bottom and top layers respectively. The dashed hexagon represents the super-lattice BZ. b$_1$, b$_2$, $\tilde b_1$, and $\tilde{b}_2$ are the reciprocal lattice vectors of the top and bottom layers respectively. A Dirac point of the bottom layer at K coupled to the top layer Dirac point k$_r$ by three distinct momentum conservation processes through g$_1$, g$_2$, and g$_3$.}
	\label{figs2}
\end{figure}
%%============================% 
%%%%%%%%%%%%%%%%%%%%%%%%%%%%%%%%%%%%%%%%%%%%%%%%%%%%%%%%%%
 
Figure.~\ref{figs2} shows the Brillouin zone (BZ) of a TBG with $\theta_c = 38.21^\circ$. Red and Blue hexagons represent the BZ of the bottom and upper layers respectively. 
In this case, the states of a Dirac cone at the bottom layer at K are coupled with the states of the Dirac cone K$_r$ of the upper layer by three distinct momentum conversation processes with the largest coupling amplitude $w=t_{|\bf k_D + b_1 + b_2 |}$. 
The Dirac cone at K of the bottom layer couples to the K$_r$ of the upper layer through reciprocal vectors given by,
g$_1 = (\bf G_1$, $\bf \tilde{G}_2) = (b_1, \tilde{b}_1 + \tilde{b}_2 )$, 
g$_2 = (\bf G_2$, $\bf \tilde{G}_2) = (- 2b_1 - 2b_2, -\tilde{b}_1 - 2\tilde{b}_2 )$, and
g$_3 = (\bf G_3$, $\bf \tilde{G}_3) = (- b_1 + b_2, -2\tilde{b}_1 )$ as shown in Fig.~\ref{figs2}.
Then the coupling Hamiltonian approximately becomes,
 \begin{equation} \label{eqs7}
 H_{\bf k,\tilde k}^{\alpha \beta} = w \sum_{i=1}^3 e^{i \bf G_i \cdot (\tau^\alpha + d)} e^{-i \bf  \tilde G_i \cdot\tau^\beta} 
 \end{equation}
The Hamiltonian for the external electric field is written as $H_E = \text{diag}(E, E,-E,-E)$.


\section*{S5. Second-order perturbation theory }
We use the above Hamiltonian to derive a low-energy Hamiltonian by using a second-order perturbation theory under an external electric field for a slight shift ($d_x,d_y$) around the EAB configuration. 
The Hamiltonian becomes,
\begin{widetext}

\begin{align}
H_{d_x,d_y}(k_x,k_y)= &
\frac{8 \pi   v (d_y k_x -d_x k_y)}{9 \sqrt{7}}  \sigma_0
+ \left(\frac{v^2 (k^2_x - k^2_y)}{w} + \frac{2 \pi  d_y w}{9}\right) \sigma_1
+\left(-\frac{2 k_x k_y v^2}{w} -  \frac{2 \pi d_x w}{9}\right) \sigma_2  \\ \nonumber
& + \left(E + \frac{4 \pi  v (d_x k_x + d_y k_y)}{3 \sqrt{21}}\right) \sigma_3 . 
\end{align}

We then rewrite the above Hamiltonian as,
\begin{align} \label{eqs9}
 H_{d_x,d_y}(k_x,k_y)  =  m_0~({\bf d \times k}) \sigma_0 + (\alpha (k_x^2 - k_y^2) + m_1 d_y))\sigma_1  - (2\alpha ~ k_x k_y  + m_2 d_x )\sigma_2  + (E+ m_3 ~ {\bf d \cdot k}) \sigma_3,
\end{align}

where $m_0=\frac{8 \pi \nu}{9\sqrt{7}}$,
${\bf d} \times{\bf k} = d_y k_x - d_x k_y$, 
$\alpha=\frac{\nu^2}{w}$, 
$m_1=m_2=\frac{2 \pi w}{9}$, 
$m_3 = \frac{4 \pi \nu }{3\sqrt{21} }$, and
${\bf d} \cdot {\bf k} = d_x k_x + d_y k_y$. 

For $d_x=0$ and ignoring the $\sigma_0$ term (as it only shifts the bands in energy scale), the above Hamiltonian becomes,
\begin{align} \label{eqs10}
 H_{0,d_y}(k_x,k_y)  =  (\alpha (k_x^2 - k_y^2) + m_1 d_y))\sigma_1  - 2\alpha ~ k_x k_y \sigma_2  + (E+ m_3 ~ d_y k_y) \sigma_3.
\end{align}

We use Eq.~\ref{eqs10} in the main paper for further studies.

\end{widetext}

%%%%%%%%%%%%%%%%%%%%%%%%%%%%%%%%%%%%%%%%%%%%%%%%%%%%%%%
%%======= moier theory  ===========% 
\begin{figure*}[t!]
	\centering
	\includegraphics[width=0.8\textwidth]{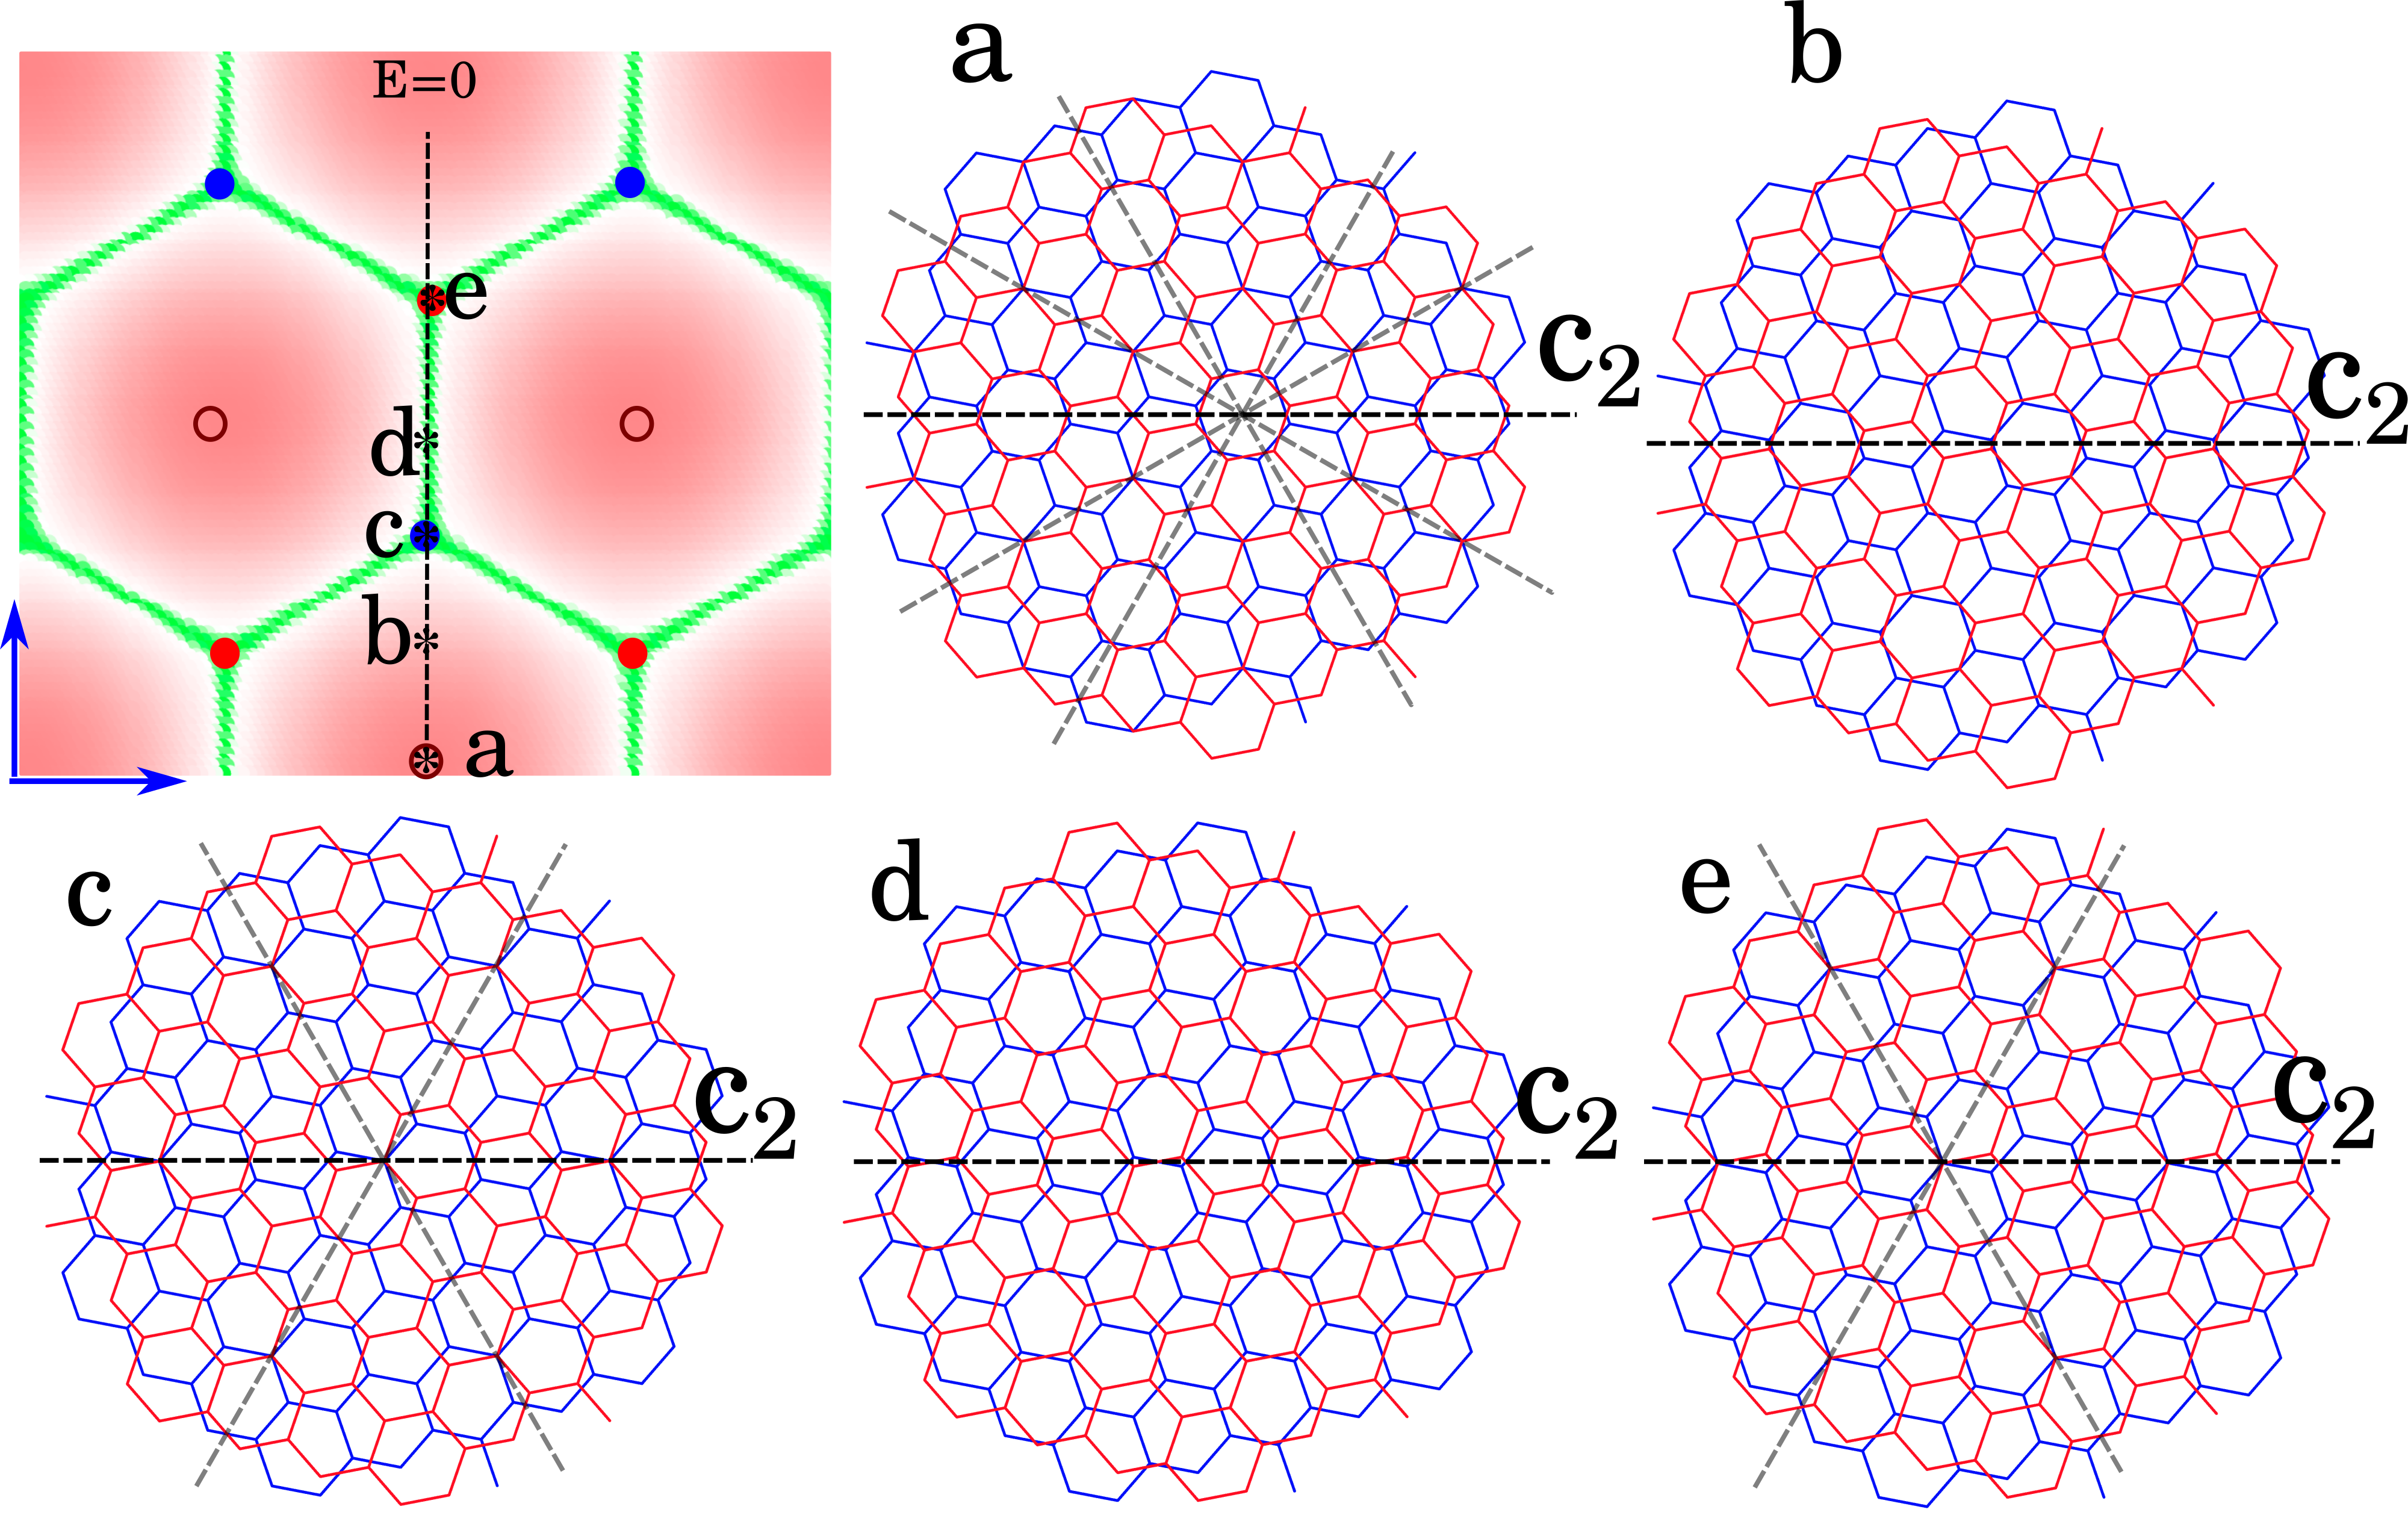}
	\caption{ Symmetries of local structure in the domain wall network. \qq{a}, \qq{b},\qq{c},\qq{d}, and \qq{e} are the chosen position whose local structures are shown. }
	\label{figs3}
\end{figure*}
%%============================% 
%%%%%%%%%%%%%%%%%%%%%%%%%%%%%%%%%%%%%%%%%%%%%%%%%%%%%%%%


\section*{S6. The symmetry of the local structure }
Small twisting of two graphene layers from commensurate angle $\theta_c=0$ creates local AA, AB, and BA stacking configuration over a large length scale. 
This phenomenon should be true not only for $0^\circ$ but also for any $\theta_c$. 
A small twisting from $\theta_c=38.21^\circ$ creates EAA, EAB, and EBA local configurations. 
The local structures  EAA, EAB, and EBA create a domain wall network as shown in Fig.~\ref{figs3}. 
The EAA, EAB, and EBA can be constructed from one to the other by suitable shift as shown in Fig.1 in the main manuscript. For instance, to construct EAA from EAB, we have to shift one layer w.r.t other layer by a shift vector \{0, 2d$_0$\} as shown in Fig.1 (a) in the main manuscript. It is clear that the eclipsed atoms have AB (or BA) stacking similar to the AB-stacked bi-layer graphene. Suppose that the stacking of the atoms in the eclipsed atoms are in AB stacked, i.e., A sub-lattice of one layer is eclipsed by B sub-lattice of other layer. d$_0$ is the minimum amount of shift that would change the staking of the eclipsed site from AB to BA. Therefore, the EAB can be converted to EBA by d$_0$ shifting. Also, similar to the bi-layer graphene, the 2d$_0$ shift takes EAB to EAA stacking. 

The gapless domain wall modes are represented by green color and pink regions are gapped. 
In this domain wall network, two domains are smoothly connected. 
In Fig.~\ref{figs3}, we show a few local structures and their underlying symmetries. 
The local configurations are labeled by \qq{a}, \qq{b},\qq{c},\qq{c}, \qq{d}, and \qq{e} on a vertical dashed line.
The local structure at \qq{a} is exactly the EAA configuration. 
It has six in-plane two-fold rotation symmetries as shown by the dashed line. 
The black dashed line represents the $\mathcal C_{2x} : (x,y,z) \rightarrow (x,-y,-z)$ symmetry. 
Other $\mathcal {C}_2$ (gray dashed lines) can be generated by underlying three-fold two-fold rotation ($\mathcal C_{3z}$ and $\mathcal C_{2z}$) symmetries of the local structure at this position.
The local structure at position \qq{b} has only one $\mathcal C_{2x}$ symmetry. At position \qq{c}, the local structure is EAB which has three in plane $\mathcal C_{2x}$ connected by $\mathcal C_{3z}$. The local structure at position \qq{d} possesses a $\mathcal C_{2x}$ symmetry. 
At position \qq{e}, the configuration is EBA which has the same symmetry configuration as EAB at position \qq{c}. 

 

\section*{S7. Effective theory for Domain wall network based on the local structure symmetry }
We derive an effective theory for the domain wall network states by a Hamiltonian construction near EAB/EBA, purely based on the symmetry of local structures of the domain wall network. 
As we have discussed in the previous section that the locus of all local structures on a line joined by the positions \qq{a}, \qq{b}, \qq{c}, \qq{d}, and \qq{e} has $\mathcal{C}_{2x}$ symmetry.
Aditionnaly, the positions \qq{c} (EAB) and positions \qq{e} (EBA) possess $\mathcal{C}_{3z}$ symmetry.
 We choose $\mathcal{C}_{2x}$ = $\sigma_x$, and $\mathcal{C}_{3z}$ = $e^{i \frac{2\pi}{3} \sigma_z }$. 
We write a $\mathcal{C}_{2x}$ symmetric Hamiltonian up to the second order of momentum which is given by

\begin{widetext}
\begin{align}
H= (\alpha~k_x^2 + \beta~k_y^2 + p_1~k_x + p_2 )\sigma_x + (\gamma~k_x k_y + p_3~k_y) \sigma_y  + (p_4~k_x k_y + p_5~k_y)\sigma_z
\end{align}
\end{widetext}
 
 where $\alpha$, $\beta$, $\gamma$ and $p_i$ are the constants. 
In general, the $H$ does not support a gapless solution for arbitrary $k_x$ and $k_y$. 
However, we can choose two special cases for $k_x=0$ and $k_y=0$ momentum lines. For $k_x=0$, the solution of $H$ is $E_\pm = \pm \sqrt{(\beta~k_y^2 + p_2)^2 + p_3^2 + p_5^2 }$ which does not support any protected gapless solutions. On the contrary, $k_y=0$ supports either two gapless solutions or no solutions depending on the sign of the $p_i$.
For instance, for $k_y=0$, Hamiltonian becomes $H=(\alpha~k_x^2 + m_1~k_x + m_2)\sigma_x$. Two gapless solutions can be obtained at $k_x = \pm k_0 = \frac{-p_1 \pm \sqrt{p_1^2 -4\alpha p_2} } {2\alpha}$ if $p_1^2 > 4 \alpha p_2$, and two imaginary solutions if $p_1^2 < 4 \alpha p_2$. These gapless (imaginary) solutions represent the gapless domain wall modes (gaped modes away from the domain wall). 
$p_1^2 = 4 \alpha p_2$ enforces a critical band touching point and then reopens a gap with two Dirac points for $p_1^2 > 4 \alpha p_2$  at $\pm k_0$.
The critical touching points at EAB also possess addition $\mathcal{C}_{3z}$ symmetry when $p_i = 0$, $\beta = -\alpha$ and $\gamma = -2\alpha$ which enforce a quadratic degeneracy at EAB.
The exact same conclusions for the domain wall modes have been drawn in the main paper using effective perturbation theory.  




\section*{S8. Ribbon construction }
In this section, we show the ribbons for which we calculate domain wall modes in Fig.2 in the main manuscript. Although we consider a very large ribbon length in the calculations, here we show a small length for a better representation as shown in Fig.~\ref{fig-S4}.
%%%%%%%%%%%%%%%%%%%%%%%%%%%%%%%%%%%%%%%%%%%%%%%%%%%%%%%
%%======= ribbon  ===========% 
\begin{figure*}[t!]
	\centering
	\includegraphics[width=\textwidth]{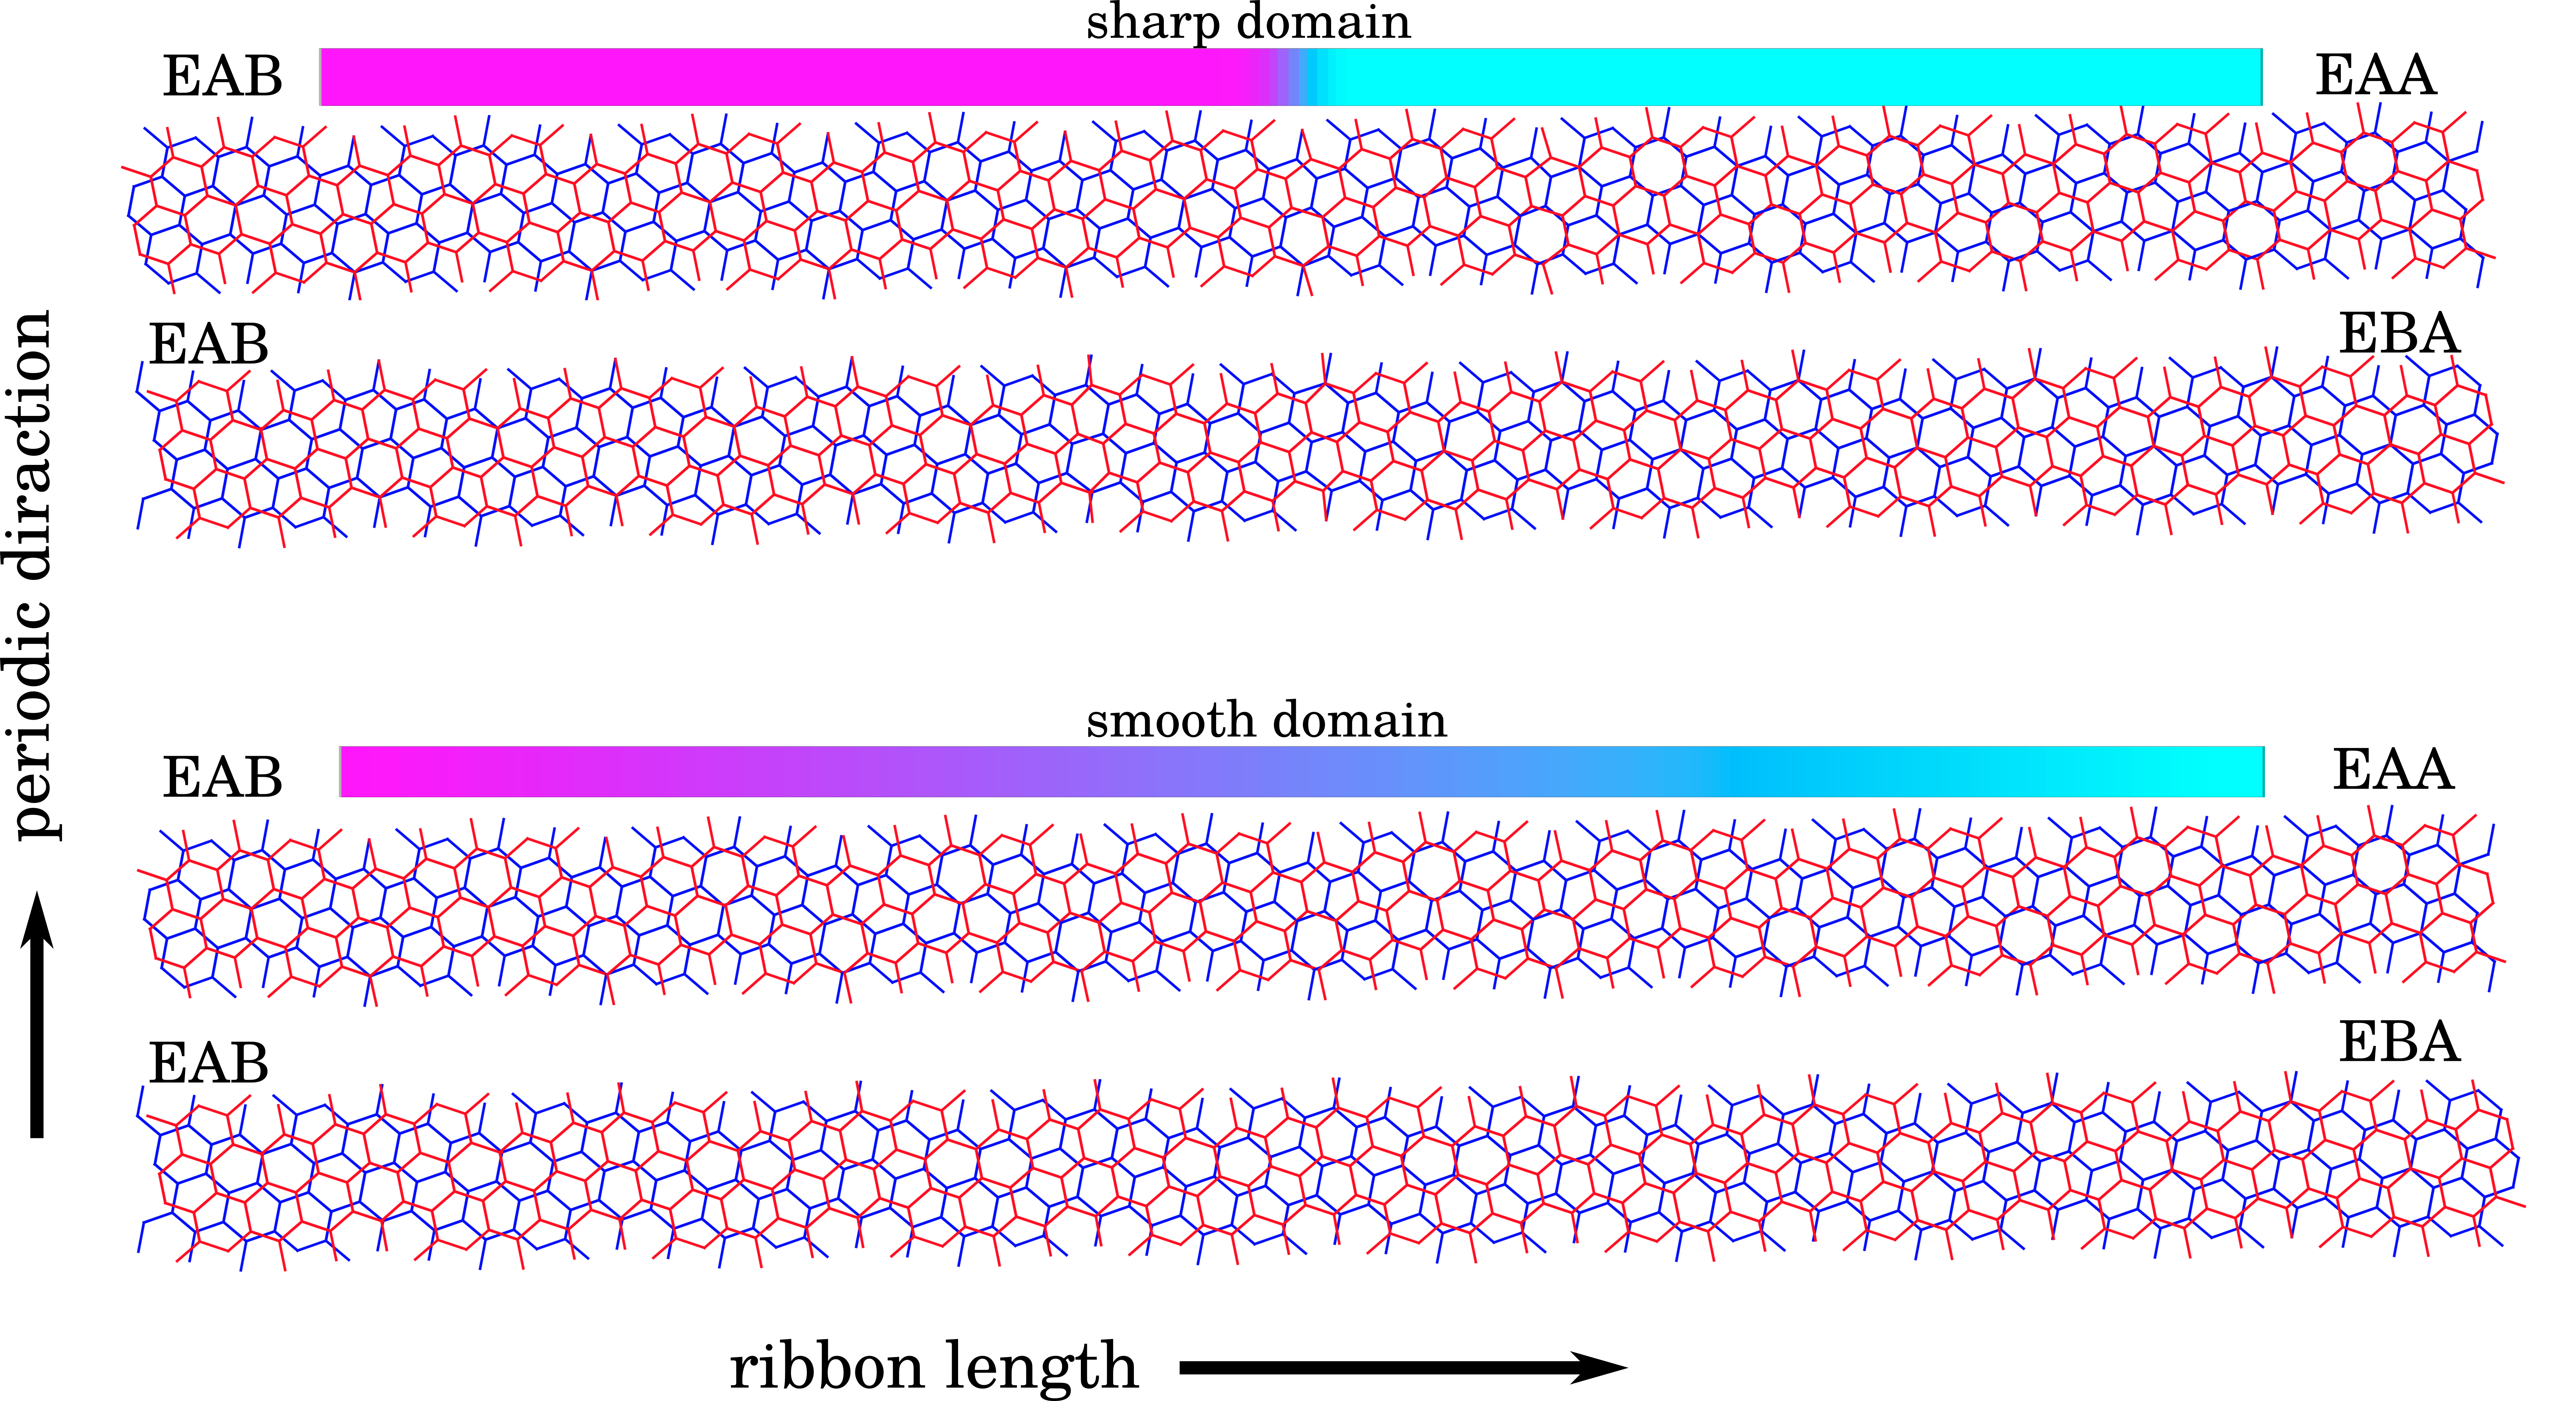}
	\caption{Sharpe domain (top panel) and smooth domain (bottom panel) between EAB-EAA and EAB-EAA configurations. }
	\label{fig-S4}
\end{figure*}
%%============================% 


\section*{S9. Band structures of additional materials }
In this section, using DFT band structure calculations, we predict a few more twisted material platforms to realize our theory on the valley and sub-valley Hall effect and the domain wall states. Here we propose that the twisted bilayer $\alpha$-graphyne should show properties similar to the twisted bilayer graphene at large angles.  Figure.~\ref{fig-s5} shows the band structure of EAB and EAA configurations of twisted bilayer $\alpha$-graphyne at $\theta_c$=38.21$^\circ$. The band structures show quadratic band touching and an energy gap for EAB and EAA similar to the twisted bilayer graphene. Therefore, our theory is also applicable in twisted bilayer $\alpha$-graphyne. Interestingly, very recent work shows that the gaped EAA configurations of twisted bilayer $\alpha$-graphyne support the real Chern topological insulator phase \cite{graphyne}. This conclusion is also aligned with the topological phase of the EAA configuration of twisted bilayer graphene. 
We also found another study on twisted bilayer kagome material. The band dispersion of the twisted bilayer kagome resembles the band structures of twisted bilayer graphene at large angles\cite{kagome}. Therefore, we expect that the twisted bilayer kagome should also show similar phenomena that we proposed in the twisted bilayer graphene. 


%%%%%%%%%%%%%%%%%%%%%%%%%%%%%%%%%%%%%%%%%%%%%%%%%%%%%%%
%%======= device  ===========% 
\begin{figure}[t!]
	\centering
	\includegraphics[width=0.5\textwidth]{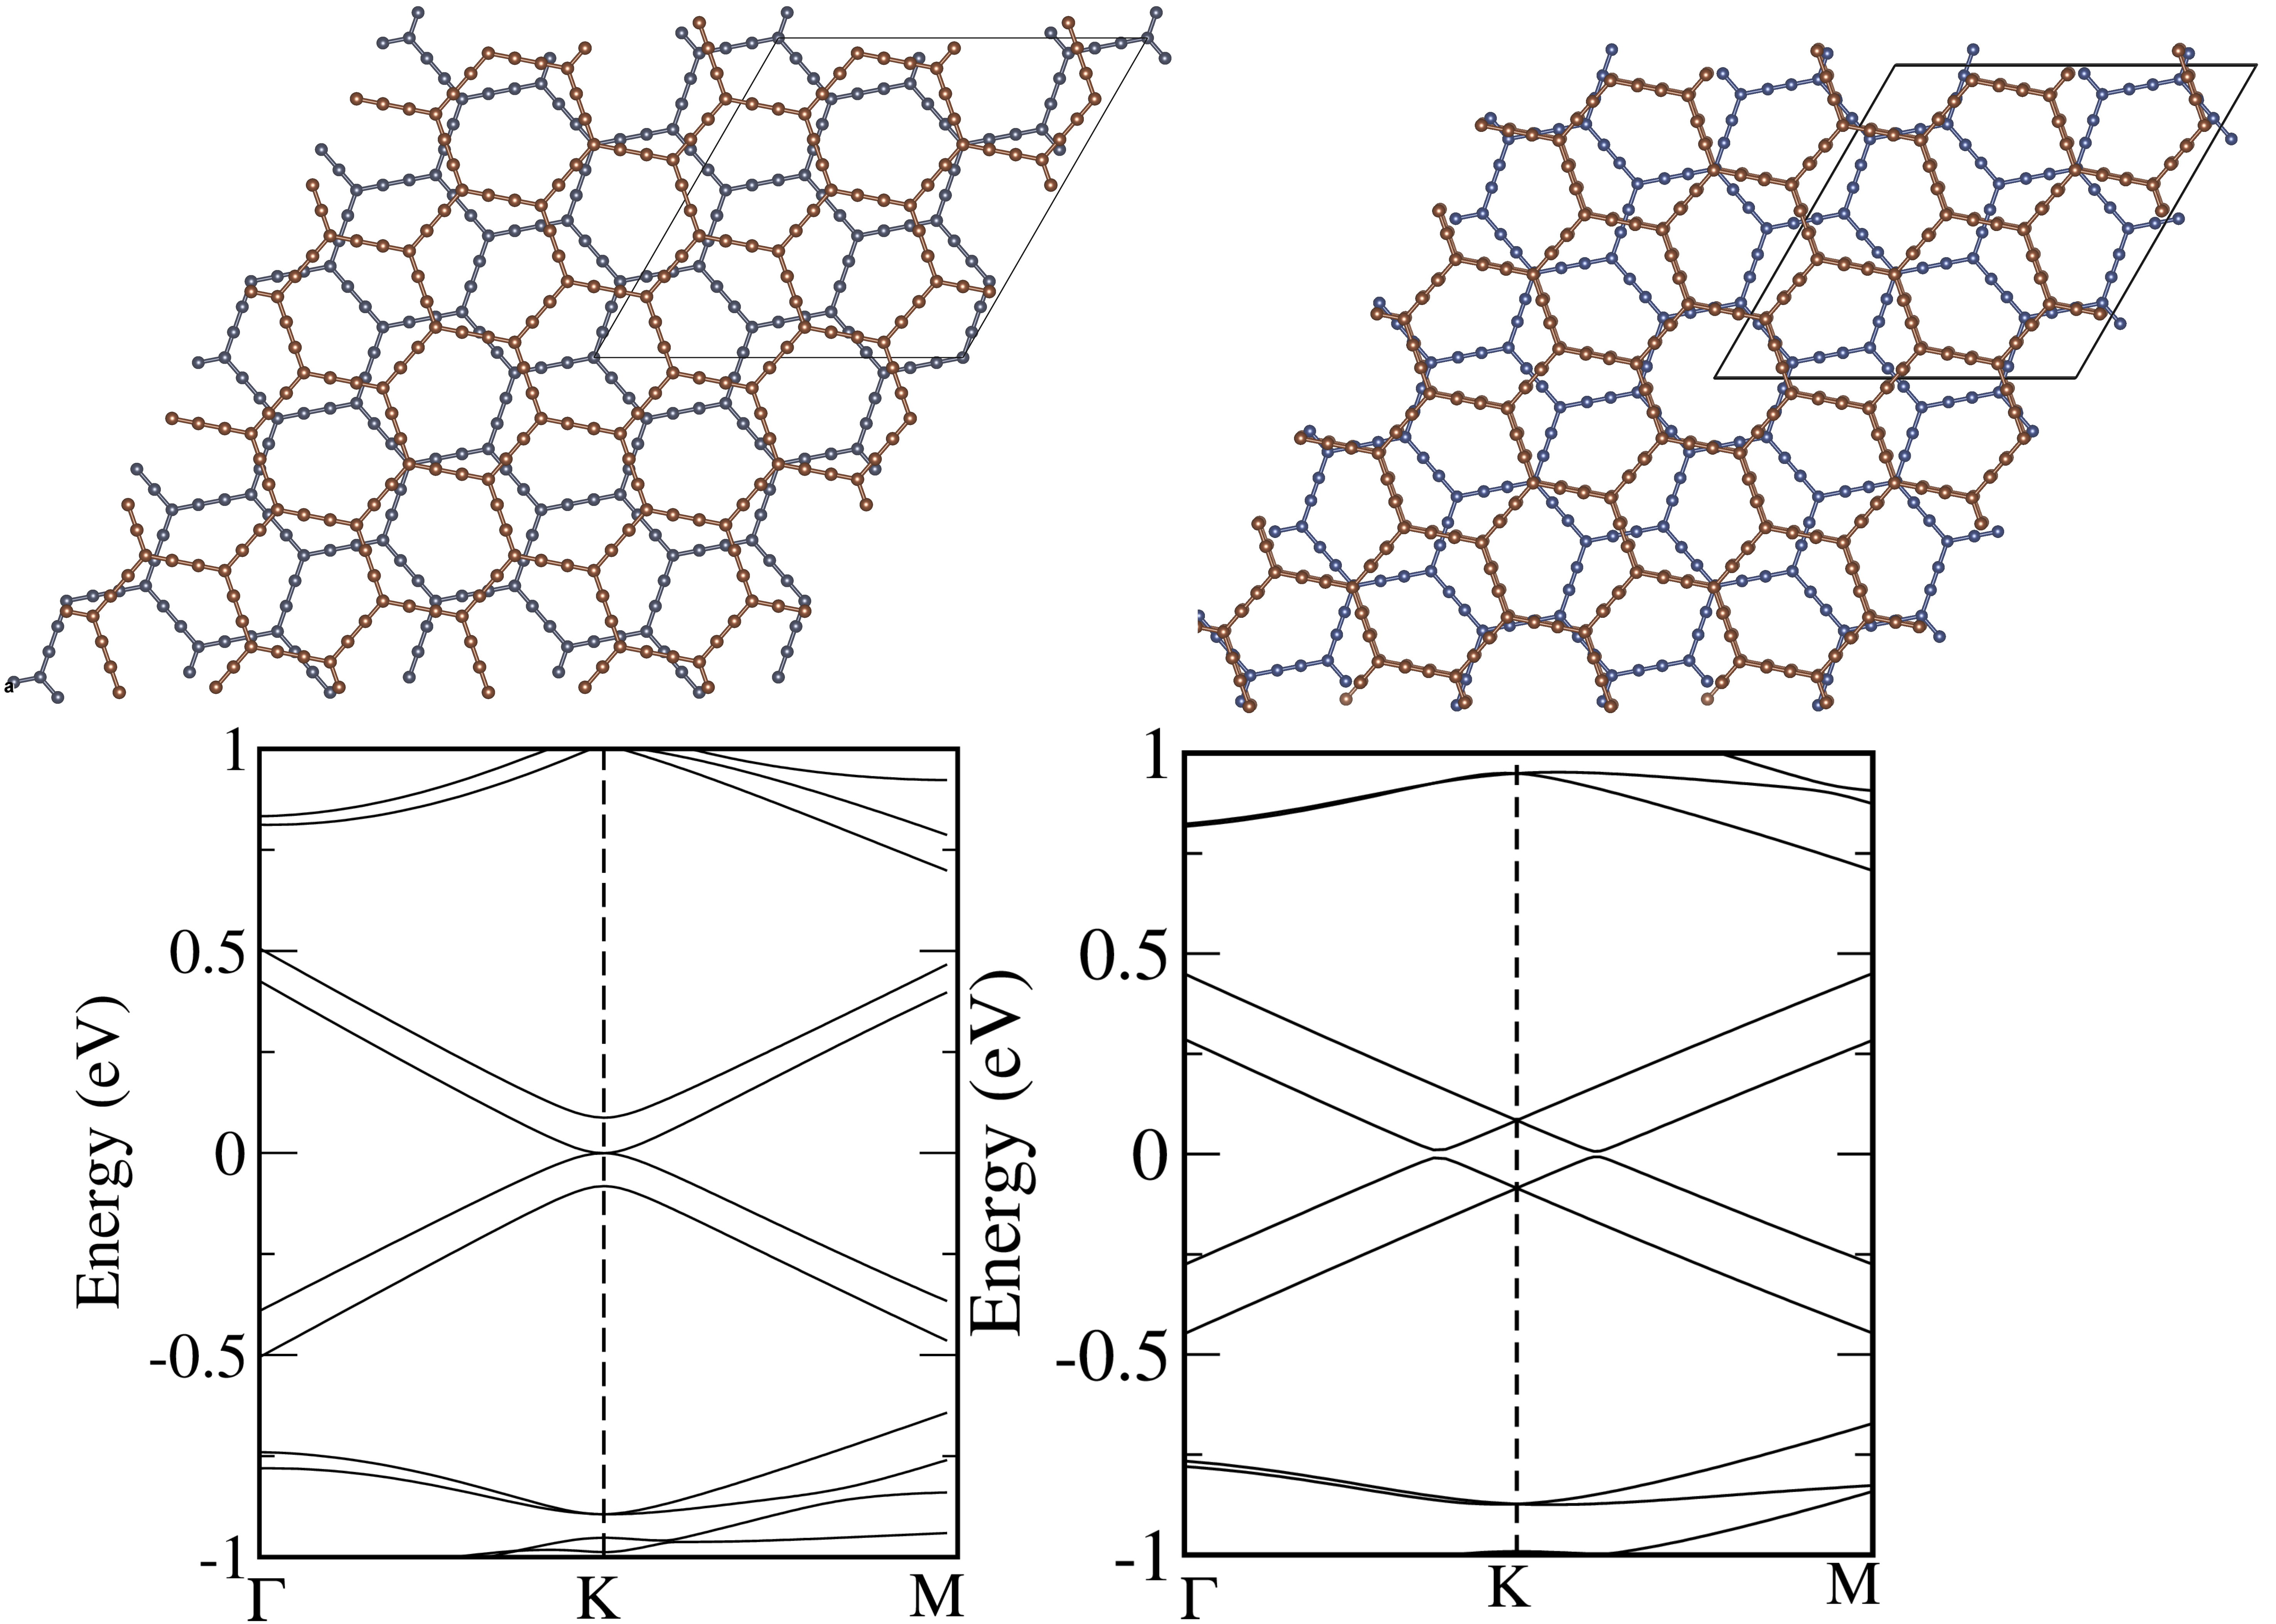}
	\caption{ EAB/EBA and EAA configurations of twisted $\alpha$-graphyne at $\theta_c$=38.21$^\circ$ (top panel). Their corresponding band structures (bottom panel).  }
	\label{fig-s5}
\end{figure}
%%============================% 



 
%%%%%%%%%%%%%%%%%%%%%%%%%%%%%%%%%%%%%%%%%%%%%%%%%%%%%%%%%%%%%%%%%%%%%
%                     Reference Page
%%%%%%%%%%%%%%%%%%%%%%%%%%%%%%%%%%%%%%%%%%%%%%%%%%%%%%%%%%%%%%%%%%%%%%

\newpage



\begin{thebibliography}{99}

%------------------DFT----------------------------

\bibitem{PEBLOCH1994} P. E. Bl\''{o}chl, Projector augmented-wave method, \PRB {\bf 50}, 17953 (1994).

\bibitem{Hafner1993} G. Kresse and J. Hafner, Ab initio molecular dynamics for liquid metals, \PRB {\bf 47}, 558(R) (1993).

\bibitem{Joubert1999} G. Kresse and D. Joubert, From ultrasoft pseudopotentials to the projector augmented-wave method, \PRB {\bf 59}, 1758 (1999).

%\bibitem{HSE} J. Heyd, G. E. Scuseria, and M. Ernzerhof, Hybrid functionals based on a screened Coulomb potential, J. Chem. Phys. {\bf 118}, 8207 (2003).

\bibitem{mlwf1} N. Marzari and D. Vanderbilt, Maximally localized generalized Wannier functions for composite energy bands, \PRB 56, 12847 (1997).

\bibitem{mlwf2} Ivo Souza, N. Marzari, and D. Vanderbilt, Maximally localized Wannier functions for entangled energy bands, \PRB {\bf 65}, 035109 (2001).

\bibitem{mlwf3} N. Marzari, A. A. Mostofi, J. R. Yates, Ivo Souza, and D. Vanderbilt, Maximally localized Wannier functions: Theory and applications, Rev. Mod. Phys. {\bf 84}, 1419 (2012).

\bibitem{w90} AA Mostofi, JR Yates, G Pizzi, YS Lee, I Souza, D Vanderbilt, N Marzari, wannier90: A tool for obtaining maximally-localised Wannier functions, Comput. Phys. Commun. {\bf 185}, 2309 (2014)

% \bibitem{greenfn1} D. H. Lee and J. D. Joannopoulos, Simple scheme for surface-band calculations., \PRB {\bf 23}, 4988 (1981).

% \bibitem{greenfn2} D. H. Lee and J. D. Joannopoulos, Simple scheme for surface-band calculations. II. The Green's function, \PRB {\bf 23}, 4997 (1981).

% \bibitem{greenfn3} M. P. Lopez Sancho, J. M. Lopez Sancho, J. M. L. Sancho, and J. Rubio, Highly convergent schemes for the calculation of bulk and surface Green functions, J. Phys. F: Met. Phys. {\bf 15}, 851 (1985).

% \bibitem{WTools} Q.-S. Wu, S.-N. Zhang, H.-F. Song, M. Troyer, and A. A. Soluyanov, WannierTools: An open-source software package for novel topological materials, Comput. Phys. Commun. {\bf 224}, 405 (2018).


%%%TB parameters%%%%%%

\bibitem{tbg1} G. Trambly De Laissardiere, D. Mayou, and L. Magaud, 
Localization of Dirac Electrons in Rotated Graphene Bilayers
Nano Lett. {\bf 10}, 804 (2010).


\bibitem{tbg2} Pilkyung Moon and Mikito Koshino, 
Optical absorption in twisted bilayer graphene,
\PRB {\bf 87}, 205404 (2013).

%%%%%%%%%%%%%%%%%%%%%%%%%


\bibitem{graphyne} Bin-Bin Liu, Xu-Tao Zeng, Cong Chen, Ziyu Chen, and Xian-Lei Sheng, 
Second-order and real Chern topological insulator in twisted bilayer 
$\alpha$-graphyne, \PRB {\bf 106} 035153 (2022). 

\bibitem{kagome} F. Crasto de Lima, and R. H. Miwa†, 
Double flat bands in kagome twisted bilayers,  
\PRB {\bf 100} 155421 (2019). 



\end{thebibliography}
\end{document}
